# Supplementary material for: Selectivity gain in olfactory receptor neuron at optimal odor concentration
Source: arXiv:2504.10401 ancillary file (2025-04-14)
Supplement: Supplementary file 1 [file diffEq_on_dt.pdf]

# Simulation of the membrane voltage evolution in the odor presence

A.K.Vidybida\*

Bogolyubov Institute for Theoretical Physics, Kyiv, Ukraine

February 25, 2025

## Abstract

Here we describe the numerical algorithm used in the program for calculating ORN's response to odor stimulation.

## 1 Model of ORN

As model ORN we use the leaky integrate-and-fire model with fluctuating conductance input similar to that used in [1]:

$$c_m \frac{dV(t)}{dt} = -g_l(V(t) - V_{rest}) - n(t)g_{OR}(V(t) - V_e), \quad (1)$$

where

$V(t)$  — is the membrane voltage (denoted in the program either as **V1** or **V2**);

$V_{rest}$  — is the resting voltage (denoted in the program as **Vrest** and read from the file **DATA.ORN**);

$c_m$  — is the total capacity of ORN's membrane (denoted in the program as **cm**);

$g_l$  — is the total leakage through it (denoted in the program as **g1**);

$V_e$  — is the reversal potential for current through open OR channel (denoted in the program as **Vexcit** and read from the file **DATA.ORN**);

$n(t)$  — is the fluctuating number of bound ORs at moment  $t$  (denoted in the program either as **n1** or **n2**);

$g_{OR}$  — is the conductance of single open OR channel (denoted in the program as **ge** and read from the file **DATA.OR**).

---

\*<http://vidybida.kiev.ua/>

The model presented in the Eq. (1) is, as usual, extended with the threshold voltage,  $V_{th}$  (denoted in the program as `Vth` and read from the file `DATA.ORN`): if  $V(t)$  exceeds  $V_{th}$ , then the ORN fires a spike and  $V(t)$  is reset to  $V_{rest}$ .

Our purpose is to run evolution as described above for some period  $T$  (denoted in the program as `T`) and to calculate the total number of spikes emitted (denoted in the program either as `fire1` or `fire2` for the odor O1 or O2, respectively).

## 1.1 Numerical algorithm

The total number of ORs bound with odor,  $n(t)$  in (1) is a fluctuating quantity simulated with the help of random number generator as described in the document `stoch_proc_simulation.pdf` in this directory. Each new value of  $n(t)$  is supplied at the beginning of each time step  $dt$  and is considered constant during the  $dt$ . Thus, transition from  $V_k \equiv V(k dt)$  to  $V_{k+1} \equiv V((k+1) dt)$  is governed by the following linear differential equation with constant coefficients:

$$\frac{dV(t)}{dt} = -\alpha_k V(t) + \beta_k, \quad (2)$$

with initial condition  $V(k dt) = V_k$ , where

$$\alpha_k = \frac{g_l + g_{OR} n_k}{c_m}, \quad \beta_k = \frac{g_l V_{rest} + g_{OR} n_k V_e}{c_m}, \quad n_k \equiv n(k dt). \quad (3)$$

Eq. (2) can be easily solved during interval  $[k dt; (k+1) dt]$ , which gives for the time dependence there:

$$V(k dt + t) = V_k e^{-\alpha_k t} + \frac{\beta_k}{\alpha_k} (1 - e^{-\alpha_k t}), \quad 0 \leq t \leq dt, \quad (4)$$

and for the next value of  $V$ :

$$V_{k+1} = V_k e^{-\alpha_k dt} + \frac{\beta_k}{\alpha_k} (1 - e^{-\alpha_k dt}). \quad (5)$$

We decide that there was a spike within  $[k dt; (k+1) dt]$  if  $V_{k+1} > V_{th}$ , and there wasn't if  $V_{k+1} \leq V_{th}$ . This is justifiable since the dependence on  $t$  in (4) is monotonous. In the case of spike, we replace  $V_{k+1}$  with  $V_{rest}$  and add 1 to the total number of spikes, `fire1` or `fire2`, before running the next time step, see files `run_trajec1.cpp`, `run_trajec2.cpp`.

The final values of `fire1` and `fire2` are used to calculate the ORN's selectivity, see file `logics_of_the_program.pdf` in this directory.

## References

- 1 Alexandre Kuhn, Ad Aertsen, and Stefan Rotter. Neuronal integration of synaptic input in the fluctuation-driven regime. *The Journal of Neuroscience*, 24(10):2345, 2004.
