# Supplementary material for: Selectivity gain in olfactory receptor neuron at optimal odor concentration
Source: arXiv:2504.10401 ancillary file (2025-04-14)
Supplement: Supplementary file 2 [file logics_of_the_program.pdf]

# Logic of the “Stochastic ORN” model / program

A.K.Vidybida\*

Bogolyubov Institute for Theoretical Physics, Kyiv, Ukraine

February 24, 2025

## Abstract

Here we describe the statement of the problem for estimating how much the ORN’s selectivity could be better, due to fluctuations in the number of odor receptor proteins bound with odor, than that of OR proteins it is populated with. Also, we sketch how the solution is organized programmatically. More details can be found in other two documents in this directory and comments in the code files.

## 1 Introduction

Theoretical estimates for an extremely simplified model of ORN suggest that selectivity  $S$  of an ORN could possibly be considerably better than the selectivity  $s$  of the OR proteins populating the ORN’s membrane, see e.g. [1]. This model / program is developed for checking such a possibility for a more realistic model of ORN. This more realistic model is described in the document `diffEq_on_dt.pdf` in this directory. See also [2] for preliminary results obtained in the framework of this model.

In order to compare  $S$  with  $s$  we give exact definitions of the both, and express the selectivity gain  $g$  as

$$g = \frac{S}{s}. \tag{1}$$

In order to find  $S$  with  $s$  given we model the odor binding-releasing process as a Markov stochastic process, and perform numerical simulation of the ORN’s response to it as it is described below, and in the `diffEq_on_dt.pdf` document in this directory.

---

\*<http://vidybida.kiev.ua/>

## 2 The logics

### 2.1 Statement of the problem

Consider two hypothetical odors O1 and O2 which are presented to a hypothetical ORN in two separate experiments at the same concentration  $c$ . For the  $c$  we use here a fixed value, which, in a sense described in [2], may be considered as optimal for having a selectivity gain. The odors have slightly different affinity with the ORN's OR proteins due to different rate constants in the following association-dissociation reaction:

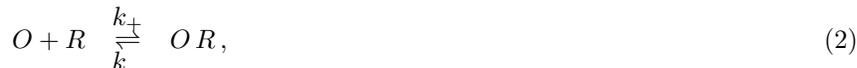

where  $R$  denotes the OR protein and  $O$  is either O1, or O2.

We express the response of OR proteins to an odor as mean in time fraction  $p$  of OR proteins bound with either analyte<sup>1</sup>:

$$p = \frac{1}{1 + K/c}, \quad (3)$$

where  $K$  — is the dissociation constant:

$$K = \frac{k_-}{k_+}. \quad (4)$$

By having the fractions  $p_1$  for O1 and  $p_2$  for O2 we calculate the OR discriminating ability (selectivity) between O1 and O2 at concentration  $c$  as follows:

$$s = \frac{p_1 - p_2}{p_1}, \quad (5)$$

assuming that  $p_1 > p_2$ .

For an ORN equipped with those OR proteins we define selectivity  $S$  as follows:

$$S = \frac{F_1 - F_2}{F_1}, \quad (6)$$

where  $F$  is the ORN's mean firing rate when exposed to either O1 or O2. By having both  $s$  and  $S$  we calculate the selectivity gain as shown in (1).

### 2.2 Realization in the program

The program is called from command line as '`./stochORN s seed`'. It reads data from the `DATA.*` files in the `data/` directory, initializes itself and makes calculations. After the run is finished, a detailed report about the run is put as `*.rep` in the `reports/` directory.

---

<sup>1</sup>we use hear "odor" and 'analyte' as synonyms.

### 2.2.1 The two odors

The program `stochORN` obtains the OR selectivity  $s$  as its command line argument. The O1 parameters are taken from the `DATA.ORN` file. And O2 parameters are chosen / calculated during initiation of the run, in such a way that the OR proteins indeed have the selectivity  $s$  between O1 and O2. Namely the program reads the rate constants  $k_+$  and  $k_-$  for the odor O1 from the `DATA.ORN` file. The second odor, O2, is assumed to have association rate constant  $k_+$  the same as does O1. The dissociation rate constant for O2,  $k_{-2}$ , is calculated in the `init2.cpp` file as:

$$k_{-2} = \frac{s \cdot k_+ \cdot c + k_-}{1 - s}. \quad (7)$$

Now we have two odors with the rate constants given in the Table 1. By

| odors | assoc. rate const., $1/(msec \cdot M)$          | dissoc. rate const., $1/msec$                                                        |
|-------|-------------------------------------------------|--------------------------------------------------------------------------------------|
| O1    | $k_+$<br>(read from the <code>DATA.ORN</code> ) | $k_-$<br>(read from the <code>DATA.ORN</code> )                                      |
| O2    | $k_+$<br>(read from the <code>DATA.ORN</code> ) | $(s \cdot k_+ \cdot c + k_-)/(1 - s)$<br>(calculated in the <code>init2.cpp</code> ) |

Table 1: Rate constants ensuring OR’s selectivity  $s$ .

substituting rate constants from the Table 1 in the Eqs. (3), (4) and (5) it can be checked that indeed the OR’s selectivity between O1 and O2 equals  $s$  exactly.

The program utilizes this idea as follows. When execution starts, it reads concrete numerical values for  $k_+$  and  $k_-$  from the file `DATA.ORN` and for concentration  $c$  — from the `DATA.RUN`. The desired trial OR’s selectivity  $s$  is supplied by user as the first command line argument. Code in the `init2.cpp` file calculates  $k_{-2}$  (denoted there as `km2`) in accordance with Eq. (7).

When initialization is finished, we have two pairs of rate constant values, for O1 and O2, such that, at concentration  $c$ , OR proteins have selectivity  $s$  between O1 and O2.

### 2.2.2 The two trajectories and ORN selectivity

Having concrete values for the association-dissociating rate constants for both O1 and O2, and concentration  $c$ , we calculate  $n(t)$ , which is how many OR proteins are bound with odor at a moment  $t$ . The moments considered have the form  $k \cdot dt$ ,  $k = 1, 2, \dots$ , where  $dt$  is the simulation time-step value read from the `DATA.RUN` file when the program starts. The trajectories are calculated in the files `run_trajec1.cpp`, `run_trajec2.cpp` for each odor. The algorithm used for calculating  $n(t)$  is described in details in the document `stoch_proc_simulation.pdf` in this directory. Simultaneously, the membrane voltage,  $V(t)$  is calculated as described in the `diffEq_on_dt.pdf` document in this directory. Every time when  $V(t)$  exceeds the firing threshold value (read

from the `DATA.ORN` file) the program registers a spike, resets  $V(t)$  to its resting value (read from the `DATA.ORN` file), but keeps  $n(t)$  as is.

The above calculations are performed in parallel both for O1 and O2 in the parent and child processes created in the `main.cpp` file.

When simulation of the stochastic processes  $n1(t)$  and  $n2(t)$  is finished, we have, both for O1 and O2, the total number of spikes, `fire1` and `fire2`, produced during the trajectory duration. The selectivity of the ORN is then calculated as

$$S = (\text{fire1} - \text{fire2}) / \text{fire1} \quad (8)$$

in the `done.cpp` file, where it is also used to calculate the selectivity gain in accordance with the Eq. (1).

### 2.2.3 Multiple sniffs / ORNs in a single trajectory

In this version of the program, a single trajectory consists of many consecutive sniffs. The sniff duration is read from the file `DATA.RUN` as `sniffDur` parameter. The number of sniffs is read from the file `DATA.RUN` as `nORN` parameter.

The purpose of this approach might be considered as an attempt to gather sufficient amount of statistics about a single ORN. We would prefer another interpretation: It is known, [3], that the number of ORNs expressing the same OR protein can be quite large (5000-10000) in the primary part of olfactory system. All these ORNs converge onto a single (or few) glomerulus and construct input for a single (or few) projection neuron. By using in the definition (8) the number of spikes `fire1` and `fire2`, produced in the course of the whole trajectory we gather a single sniff statistics for the set of these neurons. This explains the notation `nORN`.

### 2.2.4 Random number generation scheme used

The stochastic trajectories  $n1(t)$ ,  $n2(t)$  are produced as Markov processes with the help of pseudo-random number generators (RNG). The algorithm used is described in the document `stoch_proc_simulation.pdf` in this directory. We use a pair of the system RNG `lrand48()` in the parent and child processes and a pair of RNG from the GNU scientific library, [4]. The first system RNG is initialized in the `init1.cpp` file with a seed `seed` supplied as the second command line parameter when the program is called. It is used for the O1 odor. The second system RNG is initialized in the `init2.cpp` file with a mangled seed: `seed2 = seed*1.3`. Pseudo-random numbers obtained from the system RNGs are used for initialization of the GNU scientific library RNGs at the beginning of each sniff, see files `reset1.cpp` and `reset2.cpp`. It is the GNU scientific library RNGs which are used to produce the  $n1(t)$ ,  $n2(t)$  during each sniff. In the paper [2], it is wrongly stated that the GNU RNGs are reset only once, before the first sniff. Actually, they were initialized with fresh random numbers obtained from the pair of system generators `lrand48()` before each sniff.

## References

- 1 A. Vidybida. Harnessing thermal fluctuations for selectivity gain. In *2022 IEEE International Symposium on Olfaction and Electronic Nose (ISOEN)*, pages 1–3, 2022, see [doc/papers/Aveiro2022.pdf](#)
- 2 A. Vidybida. Selectivity gain in olfactory receptor neuron at optimal odor concentration. In *2024 IEEE International Symposium on Olfaction and Electronic Nose (ISOEN)*, pages 1–3, 2024, see [doc/papers/Grapevine2024.pdf](#)
- 3 K. J. Ressler, S. L. Sullivan, and L. B. Buck. Information coding in the olfactory system: evidence for a stereotyped and highly organized epitope map in the olfactory bulb. *Cell*, 79:1245–1255, 1994.
- 4 M. Galassi, J. Davies, J. Theiler, B. Gough, G. Jungman, P Alken, M. Booth, F. Rossi, and R. Ulerich. *GNU Scientific Library Reference Manual*. 2019.
