# Supplementary material for: Selectivity gain in olfactory receptor neuron at optimal odor concentration
Source: arXiv:2504.10401 ancillary file (2025-04-14)
Supplement: Supplementary file 5 [file Kyiv2023.pdf]

<https://doi.org/10.15407/ujpe68.4.266>

O.K. VIDYBIDA

Bogolyubov Institute for Theoretical Physics, Nat. Acad. of Sci. of Ukraine  
(14b, Metrolohichna Str., Kyiv 03143, Ukraine; url: <http://www.vidybida.kiev.ua/>)

## MAXIMIZATION OF THE OLFACTORY RECEPTOR NEURON SELECTIVITY IN THE SUB-THRESHOLD REGIME

*It is known that if odors are presented to an olfactory receptor neuron (ORN) in a sub-threshold concentration – i.e., when the average value of the number of the ORN bound receptor proteins (RPs) is insufficient for the generation of spikes, but such a generation is still possible due to fluctuations around the average value – the ORN selectivity can be higher than the selectivity at higher concentrations and, in particular, higher than the selectivity of the ORN's RPs. In this work, the optimal odorant concentration providing the highest ORN selectivity is found in the framework of a simplified ORN model, and the dependence of the highest selectivity on the total number of RPs in the ORN,  $N$ , and its threshold value  $N_0$  is derived. The effect of enhanced selectivity in the sub-threshold regime is best manifested, if  $N_0$  is close to either unity or  $N$ . It is also more pronounced at large  $N$ -values.*

*Keywords:* olfactory receptor neuron, selectivity, sub-threshold regime, fluctuations.

### 1. Introduction

The identification of substances in air by living organisms is performed via the olfactory sensory system in the form of odor reception/recognition. The olfactory system has a hierarchical organization [1]. In particular, neurons at every hierarchical level have a better selectivity and sensitivity to odors than those at the previous one (see, e.g., [2]). A better selectivity of secondary olfactory neurons in comparison with primary ones is explained by the mechanism of lateral inhibition in the olfactory bulb [3]. For low odorant concentrations, when the lateral inhibition mechanism does not work [2], another mechanism has been proposed [4], which is physically close to that considered in this work.

The primary reception of odors and the first stages of processing the relevant information are similar in most living organisms [5]. The very first neuron that responds to the odor is the olfactory receptor neu-

ron (ORN). The ORN is usually considered to be the first level in the hierarchical reception of odors. But the reception of an odor by the ORN includes two consecutive stages. The first stage is purely physical (see Section 1.1). At some parts of its surface that are exposed to the external environment, the ORN has a substantial number of identical receptor proteins (RPs). Within the same organism, there are many different types of RPs, and there are many neurons that carry RPs of the same type [6]. Because of the Brownian motion, odorant molecules can release the RP which they are bound with and bind to another RP. When binding an RP, ion channels become open in the ORN membrane. As a result, the membrane depolarizes, and there arises a receptor potential. If the depolarization is sufficient to excite and generate output impulses, the ORN sends them to secondary neurons.

A separate ORN reacts differently to different odorants (it sends impulses with different frequencies). In addition, ORNs with different RPs react differently to the same odorant. This circumstance makes it possible to create a combinatorial code that allows the distinguishing of many more odors than the number of different RP types [7].

Earlier, it was predicted theoretically [8] that if odorants are applied to the ORN at concentrations

Citation: Vidybida A.K. Maximization of the olfactory receptor neuron selectivity in the sub-threshold regime. *Ukr. J. Phys.* **68**, No. 4, 266 (2023). <https://doi.org/10.15407/ujpe68.4.266>.

Цитування: Відибіда О.К. Максимізація селективності ольфакторного рецепторного нейрона в підпороговому режимі. *Укр. фіз. журн.* **68**, № 4, 266 (2023).

lower than it is required for a stable generation of spikes (sub-threshold ones) so that only their random generation due to fluctuations is possible, the ORN selectivity can be substantially enhanced. In this paper, possible ORN parameters and concentrations that provide the maximum enhancement of selectivity are estimated. At the same time, an extremely simple ORN model is used, which takes into account only the statistics of the binding-release process of odorant molecules by receptor proteins. Therefore, the obtained results do not pretend to be an adequate description of the phenomena in the biological ORN. They can be interpreted only as a hint of what parameter values could improve the selectivity as much as possible. The estimates made here can be used for setting up experiments with real neurons and under conditions of low odorant concentrations in order to provide the maximum selectivity, as well as for designing artificial chemosensors.

### 1.1. Primary reception of odors

From the physical point of view, the primary reception of an odorant molecule in the olfactory system occurs in the course of the association-dissociation of this molecule with the receptor protein. In most cases, the association-dissociation reaction runs according to the following scheme:

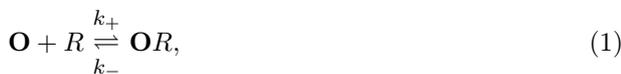

where  $\mathbf{O}$  is the odorant molecule, and  $R$  is the receptor protein. This is the first step in the odor reception process. It results in that some of receptor proteins will be occupied by the odorant molecules, whereas the remaining RPs will remain free. The quantitative measure of this result is the ratio

$$p = \frac{n}{N} \quad (2)$$

between the number of occupied RPs,  $n$ , and the total RP number,  $N$ , in a single ORN. If, in the course of two independent experiments, an ORN receives two different odorants with the same concentration, but the fractions of occupied RPs are different, then the RP can distinguish between those two odors, i.e., it is selective with respect to them. If the fractions are equal, the RP is not able to do this. In the latter case, the corresponding ORN will also be not able to

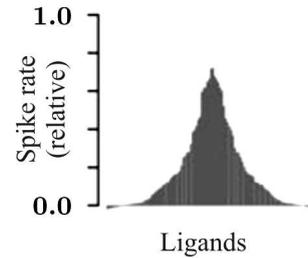

**Fig. 1.** Example of different frequencies of output spikes generated by an ORN for one type of RPs stimulated by different odorants. Adapted from [9] (through Creative Commons public license, <https://creativecommons.org>). See also [5, Fig. 3]

distinguish between the indicated two odorants, because the depolarizing transmembrane current, which governs the rate of spike generation by the neuron, depends on the number of occupied RPs.

#### 1.1.1. ORN selectivity

The ultimate result of the odor reception by an olfactory receptor neuron is the generation of output impulses by this neuron. Most ORNs generate impulses as a response to lots of various odors: they are generalists rather than specialists. The ability of ORNs to distinguish between two odorants manifests itself in the different impulse frequencies, if the odorants are presented in the same concentration in two independent experiments. For a set of odorants that a single ORN reacts to, a curve that conditionally characterizes the ORN selectivity can be plotted (see Fig. 1).

We now put a question: Is the selectivity of ORN identical to that of its receptor proteins? It is clear that the larger the share of RPs bound to odorant molecules, the larger the depolarization of the ORN excitatory membrane and the higher the generation frequency of output spikes by the ORN. This relation connects the selectivity of the ORN with that of its RP. However, in view of complicated intermediate mechanisms of chemo-electrical transduction from the RP binding-release to the creation of receptor potential and further to the spike generation, there is no reason to equate the selectivities of RPs and ORN expressing those proteins.

The aim of this work is to elucidate at which ORN parameters and odorant concentrations one may expect the highest selectivity of the ORN assuming the random binding-release of its RPs. For this purpose, the simplest ORN model was applied, where all inter-

mediate stages of chemo-electrical transduction giving rise to the spike generation are replaced by the fact of reaching the threshold value by the number of bound RPs. The reception regime in which fluctuations in the number of bound RPs substantially affect the spike generation, the sub-threshold regime, is also considered (Section 2.1.1). Previous results obtained in the framework of this model [8] showed that it is possible to obtain the selectivity of ORN in the sub-threshold regime that considerably exceeds the selectivity of its RPs.

## 2. Methods

### 2.1. Membrane-free ORN model

The ORN model analyzed here includes only the events that happen at the outer ORN surface in the course of the interaction between the ORN's RPs and odorant molecules. This model is similar to that discussed in work [10], but is even simpler, because it does not consider the passage of odorant molecules through the mucus of olfactory epithelium. In the framework of this model, the ORN is characterized by the total number  $N$  of identical receptor proteins incorporated into its membrane, and the threshold number  $N_0 < N$ . If the number of bound RPs is less than  $N_0$  ( $n < N_0$ ), then the ORN does not generate spikes. In the opposite case, the ORN generates spikes at a constant frequency  $f$  (cf. [10, Section "Olfactory threshold"]).

It should be noted that the application of this model implies that the binding of one RP with an odorant molecule opens one ion channel. This is the case for the ORN of insects, where the receptor proteins are heteromeric ligand-gated ion channels [11]. In the ORN of more complicated organisms, intermediate biochemical events take place between the RP binding and the opening of ion channels, and, as a result, the binding of one RP provides the opening of several channels, which are structurally separated from the RP (see, e.g., [12]). Those intermediate events are an additional source of fluctuations and require the additional analysis in a separate paper.

#### 2.1.1. Sub-threshold regime

To simplify calculations, it is assumed here that the ORN generates output impulses at a constant fre-

quency  $f$  irrespective of how much the threshold  $N_0$  is exceeded. This assumption is a substantial deviation from reality, if the odorant concentration is high, and the number of bound RPs,  $n$ , permanently exceeds the threshold value  $N_0$ . In this case, the growth of  $n$  increases the frequency of output impulses. But, in this work, the consideration is focused on low concentrations, when the average number of bound RPs is less than the threshold value, and the threshold is reached for short time intervals due to fluctuations (see Section 2.3). It is assumed that either one or no impulse can be generated during the permanent stay above the threshold. In this regime, the average frequency of output impulses is governed by the probabilistic characteristics of the threshold crossing, rather than the degree of threshold exceedance.

In order to strictly substantiate that the sub-threshold regime described above is possible, it is necessary to know the temporal characteristics of the stochastic process of RP binding-release and the kinetics of the process of generating output impulses by the excitable neuronal membrane. Those parameters include the reaction rate constants, the conductivity of the channels that become open at the RP binding, and the electrical characteristics of the membrane. Those parameters can be taken into account in numerical simulations. In this work, we do not specify them and intend to do so in the future.

### 2.2. Definition of selectivities

The selectivity of RP and ORN can be defined in various ways. Here, we follow the definitions from work [8]. They exclude the consideration of the concentration and the dissociation reaction constant  $K$  [see Eq. (1) below], and the consideration is based on the fraction  $p$  of bound RPs (2). This approach is justified for two reasons. First, it is simpler to deal with  $p$ . Besides, formula (8) given below provides an unambiguous relationship between  $K$  and  $p$ , if the concentration  $c$  is fixed, or between  $c$  and  $p$  if the dissociation constant  $K$  is fixed. Second, the olfactory neuron has no access to the  $K$ - and  $c$ -values, whereas the information about the total RP number  $N$  and the number  $n$  of bound RPs on the neuron surface [which, according to formula (2), is equivalent to knowing the  $p$ -value] is exactly what is subjected to a further processing in the ORN and invokes the generation of output impulses.

The selectivity of RPs with respect to two odorants  $\mathbf{O}_1$  and  $\mathbf{O}_2$  is defined as follows. If  $\mathbf{O}_1$  and  $\mathbf{O}_2$  are presented to the ORN at the same concentration  $c$  in two independent experiments, and if different  $p$ -values,  $p_1$  and  $p_2$ , are observed at that, then this RP can distinguish between those two odorants. For definiteness, let  $p_1 > p_2$ , i.e.,

$$p_1 = p_2 + \Delta p, \quad \Delta p > 0. \quad (3)$$

Then the RP selectivity can be defined as follows:

$$S_R = \frac{\Delta p}{p_1}. \quad (4)$$

For the entire ORN, its reaction to the odor manifests itself as the generation of output impulses. We may expect that, owing to Eq. (3), the average impulse frequency  $F$  will be higher for  $\mathbf{O}_1$ , i.e.,

$$F_1 = F_2 + \Delta F, \quad \Delta F > 0. \quad (5)$$

Then the ORN selectivity can be defined as follows:

$$S_{\text{ORN}} = \frac{\Delta F}{F_1}. \quad (6)$$

By analogy with [10], if we assume that, at high odorant concentrations, when the number of occupied RPs permanently exceeds the excitation threshold, the ORN response is proportional to the number of occupied RPs, then the ORN selectivity will be equal to the selectivity of its RPs. Indeed, in our case, the ORN response is the average impulse frequency  $F$ . If  $F$  grows proportionally with  $n$ , then

$$S_{\text{ORN}} = \frac{N\Delta p}{Np_1} = \frac{\Delta p}{p_1} = S_R. \quad (7)$$

Therefore, for concentrations providing a permanent exceedance of the excitation threshold, the ORN selectivity in the simple transduction model is identical to the selectivity of its RPs.

If the odorant concentration is sub-threshold, and if the  $N_0$  threshold is exceeded due to fluctuations during short time intervals, then the ORN response will be determined by the fraction of time the number of bound RPs spends above the excitation threshold. Below, we analyze how the differences between the statistics of random threshold crossings for the  $\mathbf{O}_1$  and  $\mathbf{O}_2$  odorants determine the ORN selectivity.

### 2.3. Primary-reception fluctuations

Since the primary reception of odor by a receptor neuron is performed through the binding and release of odorant molecules by the neuron's receptor proteins, this event is inevitably random. As a result, secondary signals about the odor, such as the membrane (receptor) potential or the transmembrane current, will also be random. Fluctuations of the transmembrane current in the ORN of the amphibian *Ambystoma tigrinum* were observed experimentally [13]; minimum odorant concentrations,  $10^{-10} \div 5 \times 10^{-7} \div 10^{-5} \text{M}$ , were used at that. The olfactory receptor neurons of amphibians have a more complicated mechanism of chemo-electrical transduction than in the case of insects (see, e.g., [12]); in particular, it allows the temporal integration of weak stimuli [13]. In this work, in the framework of the simplified ORN model, we do not consider the possibility of the temporal integration.

When an odorant  $\mathbf{O}$  is applied to an ORN, the RPs of the latter, due to the Brownian motion, randomly bind  $\mathbf{O}$  molecules and get released from them. Here, it is assumed that the random behavior of a separate RP is independent of other RPs. After the completion of transient processes, every RP belonging to a certain ORN can be bound to an  $\mathbf{O}$  molecule with a certain probability. Note that this probability is equal to  $p$  defined in Eq. (2). If the concentration  $c$  of the applied odorant  $\mathbf{O}$  and the dissociation constant  $K$  for the association-dissociation reaction (1) between  $\mathbf{O}$  and RP are known, then, according to the known formula (cf. [14, Eq. (3)] and [10, Eq. (4)]),

$$p = \frac{1}{1 + K/c}. \quad (8)$$

For the model described in Section 2.1, it is important to know the probability  $\mathbf{P}$  of that the number of bound RPs exceeds the threshold value  $N_0$  or reaches it provided that the odorant applied to the ORN ensures a certain fraction  $p$  (on average) of occupied RPs. Since, as was indicated above, this fraction is also the probability of that a single RP is bound to an odorant molecule, then, if separate RPs are statistically independent, the sought probability  $\mathbf{P}$  of reaching/exceeding the threshold can be calculated using the known formula (see, e.g., [15, Chap. 3, Eq. (1)])

$$\mathbf{P}(N, N_0, p) = \sum_{k=N_0}^N \binom{N}{k} p^k (1-p)^{N-k}. \quad (9)$$

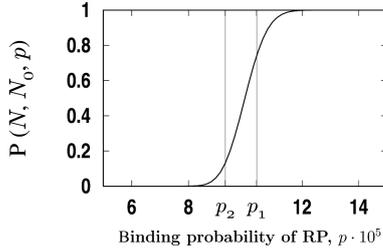

**Fig. 2.** The probability of reaching the threshold,  $\mathbf{P}(N, N_0, p)$ , for  $N = 2\,500\,000$  and  $N_0 = 250$ . Here,  $p_2 = 0.9296 \times 10^{-4}$ ,  $p_1 = 1.040 \times 10^{-4}$ ,  $S_R = 0.1$  [see Eq. (4)], and  $S_{ORN} = 0.8$  [see Eqs. (6) and (11)]. The values for  $N$  and  $N_0$  were approximately chosen on the basis of the data for the moth *Antheraea polyphemus* from work [16]

In the described approach, the quantity  $\mathbf{P}(N, N_0, p)$  is the probability of that the threshold will be reached/exceeded at some time moment, and the frequency  $f$ , which was introduced in Section 2.1, is a dimensional multiplier, which makes it possible to calculate the average frequency of output impulses,

$$F = f \mathbf{P}(N, N_0, p). \quad (10)$$

The value of  $f$  is nonessential for the definition of selectivity (6),

$$S_{ORN} = \frac{\mathbf{P}(N, N_0, p_1) - \mathbf{P}(N, N_0, p_2)}{\mathbf{P}(N, N_0, p_1)}. \quad (11)$$

### 3. Results

#### 3.1. Optimal concentration

Expression (9) for  $\mathbf{P}(N, N_0, p)$  and expression (10) for  $F$  depend on  $p$  in a “sigmoid” manner, i.e., they first grow slowly, then enter the interval with a rapid growth, and afterward slowly saturates to the corresponding constant value. Taking into account that  $p$  increases monotonically with  $c$  [see Eq. (8)], the dependences of  $\mathbf{P}(N, N_0, p)$  and  $F$  on  $c$  will also be qualitatively the same. If the odorants  $\mathbf{O}_1$  and  $\mathbf{O}_2$  have almost the same affinity to the RP, then the corresponding values of  $p_1$  and  $p_2$  will be very close to each other, which means a low selectivity of RP with respect to those odors. If the concentration of odorants is such that  $p_1$  and  $p_2$  fall into the interval of a rapid  $\mathbf{P}(N, N_0, p)$  growth, one may expect a large difference between the average frequencies of ORN impulses for those two odors [see Eq. (10)]. This will mean a better ORN selectivity. This situation is illustrated in Fig. 2.

To determine the optimal values of  $p$  and  $c$ , we have to find the point  $p_0$ , where the  $p$ -derivative of  $\mathbf{P}(N, N_0, p)$  is maximum. This derivative equals

$$\begin{aligned} \frac{d}{dp} \mathbf{P}(N, N_0, p) &= \\ &= \frac{N!}{(N_0 - 1)!(N - N_0)!} p^{N_0 - 1} (1 - p)^{N - N_0}. \end{aligned} \quad (12)$$

To find its maximum, expression (12) has to be differentiated once more,

$$\begin{aligned} \frac{d^2}{dp^2} \mathbf{P}(N, N_0, p) &\sim \\ &\sim p^{N_0 - 2} (1 - p)^{N - N_0 - 1} (N_0 - 1 - p(N - 1)) = 0. \end{aligned} \quad (13)$$

(here, the multiplier independent of  $p$  is omitted). From Eq. (13), we have

$$p_0 = \frac{N_0 - 1}{N - 1}. \quad (14)$$

Therefore, the optimal concentration  $c_0$  should provide the average number of bound RPs that is below  $N_0$  and above  $N_0 - 1$ . The corresponding  $c_0$ -value is obtained from Eqs. (8) and (14),

$$c_0 = \frac{K(N_0 - 1)}{N - N_0}. \quad (15)$$

This work is not aimed at elucidating the possible mechanisms for creating the exact optimal concentration (however, see Section 4). But it is clear that the effect of enhanced selectivity will be observed in a certain interval of  $p$ -values around  $p_0$ , which is illustrated in Fig. 2.

#### 3.2. Influence of threshold magnitude

In the previous section, it was found what concentration of weakly different odorants should be for the best manifestation of the effect of ORN selectivity enhancement in comparison with that of its RPs, if the total number of RPs in the neuron,  $N$ , and the threshold value  $N_0$  are fixed. The optimal concentration provides the optimal binding probability  $p_0$  [Eq. (14)], such that the derivative of  $\mathbf{P}(N, N_0, p)$  with respect to  $p$  is largest at the point  $p_0$ . But, the manifestation of the selectivity enhancement effect depends on the absolute value of the derivative at the point  $p_0$ . This value is determined by the quantities  $N$  and  $N_0$ .

Let us elucidate how the maximum value of the derivative,  $d\mathbf{P}_{\max}(N, N_0)$ , depends on  $N_0$  at a fixed  $N$ . For this purpose, let us substitute  $p$  by  $p_0$  in formula (12). We obtain

$$\begin{aligned} d\mathbf{P}_{\max}(N, N_0) &= \left. \frac{d}{dp} \mathbf{P}(N, N_0, p) \right|_{p=p_0} = \\ &= N \binom{N-1}{N_0-1} p_0^{N_0-1} (1-p_0)^{N-1-(N_0-1)}, \end{aligned} \quad (16)$$

where  $p_0$  is given in (14). If  $N_0 = 1$ , formula (14) gives  $p_0 = 0$ . It is clear that the selectivity to odorants with zero concentration has no sense. But, the value of  $d\mathbf{P}_{\max}(N, 1)$  can give an estimate of the slope of the plot of the function  $\mathbf{P}(N, 1, p)$  in a vicinity of the point  $p = 0$ , and this may be interesting in the case of a very low concentration<sup>1</sup>. The required value can be found as the limit

$$d\mathbf{P}_{\max}(N, 1) = \lim_{p \rightarrow 0} N \binom{N-1}{0} p^0 (1-p)^{N-1} = N. \quad (17)$$

For  $N_0 = 2$ , we have  $d\mathbf{P}_{\max}(N, 2) \approx \frac{N}{e}$ .

For large  $N$  and  $N_0$ , by applying the Stirling formula to Eq. (16), we obtain the approximate value

$$d\mathbf{P}_{\max}(N, N_0) \approx N \sqrt{\frac{N-1}{2\pi(N_0-1)(N-N_0)}}. \quad (18)$$

From whence, we can see that  $d\mathbf{P}_{\max}(N, N_0)$  increases, as  $N$  grows, which is in agreement with formula (17). An example of the plot for  $d\mathbf{P}_{\max}(N, N_0)$  is shown in Fig. 3.

### 3.3. Illustrative example

To compare the selectivity of ORN with that of its RPs, selectivity plots similar to the plot shown in Fig. 1 were drawn. For this purpose, a set of 30 different  $p$ -values inherent to hypothetical odors were generated. The obtained RP selectivity plot has a wide bell-shaped form (Fig. 4, *a*). To obtain the relative frequencies of ORN spikes (Fig. 4, *b*), those 30 indicated  $p$ -values were used in formulas (9) and (10).

<sup>1</sup> Note that the ability of mice to detect some odorants at a concentration of  $10^{-11}$  M was observed experimentally [17]. The authors of work [18] gave a value of  $10^{-13}$  M for the theoretical estimate of the minimum concentration that can be detected by the olfactory system.

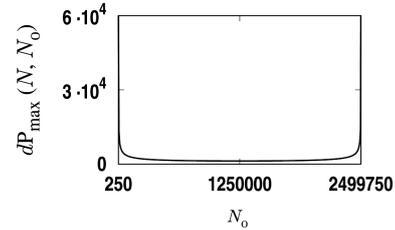

**Fig. 3.** Dependence of the maximum value of the derivative  $d\mathbf{P}_{\max}(N, N_0)$  on the threshold magnitude  $N_0$  for the fixed total number of RPs  $N = 2500000$ . The minimum of the function  $d\mathbf{P}_{\max}(N, N_0)$  equals 1262. The function values at the points  $N_0 = 250$  and  $N_0 = N - 250$  are approximately identical and approximately equal to  $63 \times 10^3$

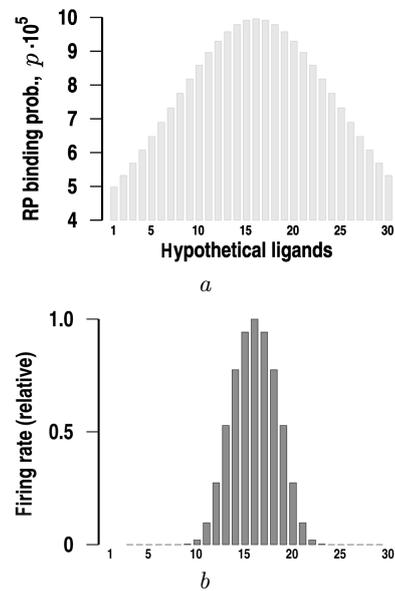

**Fig. 4.** Illustration that in the sub-threshold regime, an ORN can possess a better selectivity than its RPs: fraction  $p$  of bound RPs for a set of 30 hypothetical odors with various affinities with respect to RPs (*a*); relative frequency of the spike generation by the ORN, when the indicated hypothetical odorants are applied (*b*)

The selectivities between odors #9 and #16 from Fig. 4, which were calculated according to formulas (4) and (6), acquire the values

$$S_R = 0.178, \quad S_{\text{ORN}} = 0.998. \quad (19)$$

## 4. Discussion and Conclusions

In this work in the framework of the simplified model for an olfactory receptor neuron, two conditions are found that provide the maximum enhancement of

the ORN selectivity as compared to that of the ORN receptor proteins. The first condition is the sub-threshold regime of odor reception. It is provided by selecting the odorant concentration [Eqs. (14) and (15)]. The second condition is the minimum number  $N_0$  of bound receptor proteins required for the ORN to start the spike generation [Eqs. (16) and (18)].

From Fig. 3, it is seen that the selectivity enhancement in the sub-threshold regime is larger for ORNs with lower triggering thresholds and for very low concentrations. For real ORNs, these conditions can be satisfied only partially. First, the threshold magnitude  $N_0$  is dictated by the electrical properties of the ORN membrane and the ion channels connected with every RP. The minimum values of  $N_0$  measured for the frog ORNs are about 35 [18]. But, each bound RP in the frog ORN opens several ion channels by means of the mechanism described in work [12]. For insects, where one RP opens one channel, a threshold value of several hundreds seems to be close to reality.

Second, the total number of RPs in an ORN has to be large [see Eqs. (16)–(18)]. But, is it possible to affect the value of  $N$  fast enough? The first condition governs the way that the odor is presented, whereas the second one is responsible for the ORN structure or dynamic characteristics.

The biological olfactory system has the means to satisfy those conditions within certain limits. First, air with the dissolved odorant does not contact directly with the ORN surface, but through the mucus. The latter contains enzymes that chemically decompose the odorant molecules [19] and control the effective odorant concentration at the ORN surface. If the decomposition process takes place, the respiration rate also affects the effective concentration. Second, the level of threshold depolarization of the excitable ORN membrane depends on the ionic composition of the environment near the membrane. Changing this composition, we can affect  $N_0$ . Third, some biological mechanisms [20], with the RP internalization among them, can affect the number  $N$  of RPs at the ORN surface.

The conditions above can be satisfied in artificial neuromorphic sensors like biosensors or the electronic nose [21–25]. For such devices, the case of very high concentrations would also be of interest. As one can see from Fig. 3 (the right-hand side of the plot corresponding to large  $N_0$ -values), if the concentration

is close to the saturation, the quantity  $\mathbf{P}(N, N_0, p)$  regarded as a function of  $p$  also changes very quickly in a vicinity of  $p_0$ . However, the accurate registration of threshold crossing in the case where the threshold magnitude is equal to several millions will be problematic. On the other hand, the artificial sensor is capable of detecting the number of free receptors, which is small at high concentrations.

Some deviations of the considered model from the real ORN have been specified above. It is worth adding here that real neurons vary in time. If an ORN is subjected to a permanent exposure to the odor, its sensitivity decreases, and the adaptation phenomenon is observed [26]. The spontaneous activity of ORN in the absence of odorants [27] was also not considered here. Besides, we note that the analysis of the fluctuations of the primary response in chemical sensors is also applied beyond the receptor binding-release statistics [28, 29].

*This work was sponsored in the framework of the Fundamental research program of the Branch of Physics and Astronomy of the National Academy of Sciences of Ukraine (project No. 0120U101347 “Noise-induced dynamics and correlations in non-equilibrium systems”) and by the private American Simons Foundation.*

1. K.J. Ressler, S.L. Sullivan, L.B. Buck. Information coding in the olfactory system: evidence for a stereotyped and highly organized epitope map in the olfactory bulb. *Cell* **79**, 1245 (1994).
2. A. Duchamp. Electrophysiological responses of olfactory bulb neurons to odour stimuli in the frog. a comparison with receptor cells. *Chem. Sens.* **7**, 191 (1982).
3. W. Rall, G.M. Shepherd. Theoretical reconstruction of field potentials and dendrodendritic synaptic interactions in olfactory bulb. *J. Neurophysiol.* **31**, 884 (1968).
4. A.K. Vidybida. Possible stochastic mechanism for improving the selectivity of olfactory projection neurons. *Neurophysiology* **51**, 152 (2019).
5. J.G. Hildebrand, G.M. Shepherd. Mechanisms of olfactory discrimination: Converging evidence for common principles across phyla. *Annu. Rev. Neurosci.* **20**, 595 (1997).
6. L.B. Buck. The molecular architecture of odor and pheromone sensing in mammals. *Cell* **100**, 611 (2000).
7. B. Malnic, J. Hirono, T. Sato, L.B. Buck. Combinatorial receptor codes for odors. *Cell* **96**, 713 (1999).
8. A. Vidybida. Harnessing thermal fluctuations for selectivity gain. In *2022 IEEE International Symposium on Olfaction and Electronic Nose (ISOEN)* (2022), p. 1.

9. C.G. Galizia, D. Munch, M. Strauch, A. Nissler, Shouwen Ma. Integrating heterogeneous odor response data into a common response model: A door to the complete olfactome. *Chem. Sens.* **35**, 551 (2010).
10. A.B. Lamine, Y. Bouazra. Application of statistical thermodynamics to the olfaction mechanism. *Chem. Sens.* **22**, 67 (1997).
11. K. Sato, M. Pellegrino, T. Nakagawa, T. Nakagawa, L.B. Vosshall, K. Touhara. Insect olfactory receptors are heteromeric ligand-gated ion channels. *Nature* **452**, 1002 (2008).
12. G.V. Ronnett, Ch. Moon. G proteins and olfactory signal transduction. *Annu. Rev. Physiol.* **64**, 189 (2002).
13. A. Menini, C. Picco, S. Firestein. Quantal-like current fluctuations induced by odorants in olfactory receptor cells. *Nature* **373**, 435 (1995).
14. M. Chastrette, T. Thomas-Danguin, E. Rallet. Modelling the human olfactory stimulus-response function. *Chem. Sens.* **23**, 181 (1998).
15. B.V. Gnedenko. *Theory of Probability. 6th Edition* (CRC Press, 1998).
16. K-E Kaissling. Olfactory perireceptor and receptor events in moths: A kinetic model. *Chem. Sens.* **26**, 125 (2001).
17. E. Williams, A. Dewan. Olfactory detection thresholds for primary aliphatic alcohols in mice. *Chem. Sens.* **45**, 513 (2020).
18. V. Bhandawat, J. Reiser, K-W Yau. Signaling by olfactory receptor neurons near threshold. *Proc. Nat. Acad. Sci. USA* **107**, 18682 (2010).
19. A. Nagashima, K. Touhara. Enzymatic conversion of odorants in nasal mucus affects olfactory glomerular activation patterns and odor reception. *J. Neurosci.* **30**, 16391 (2010).
20. B. Bryche, C. Baly, N. Meunier. Modulation of olfactory signal detection in the olfactory epithelium: focus on the internal and external environment, and the emerging role of the immune system. *Cell Tissue Res.* **384**, 589 (2021).
21. K. Persaud, G. Dodd. Analysis of discrimination mechanisms in the mammalian olfactory system using a model nose. *Nature* **299**, 352 (1982).
22. B. Raman, M. Stopfer, S. Semancik. Mimicking biological design and computing principles in artificial olfaction. *ACS Chem. Neurosci.* **2**, 487 (2011).
23. C. Hurot, N. Scaramozzino, A. Buhot, Y. Hou. Bio-inspired strategies for improving the selectivity and sensitivity of artificial noses: A review. *Sensors* **20**, 1803 (2020).
24. I.S. Kucherenko, O.O. Soldatkin, S.V. Dzyadevych, A.P. Soldatkin. Electrochemical biosensors based on multi-enzyme systems: Main groups, advantages and limitations – a review. *Analyt. Chim. Acta* **1111**, 114 (2020).
25. S. Kim, R. Lee, D. Kwon, T-H. Kim, T.J. Park, S-J. Choi, H-S. Mo, D.H. Kim, B-G. Park. Multiplexed silicon nanowire tunnel fet-based biosensors with optimized multi-sensing currents. *IEEE Sensor. J.* **21**, 8839 (2021).
26. G. Antunes, A.M. Sebastião, F.M.S. de Souza. Mechanisms of regulation of olfactory transduction and adaptation in the olfactory cilium. *PLOS Comput. Biol.* **9**, e105531 (2014).
27. J. Joseph, F.A. Dunn, M. Stopfer. Spontaneous olfactory receptor neuron activity determines follower cell response properties. *J. Neurosci.* **32**, 2900 (2012).
28. J. Smulko, C-G. Granqvist, L.B. Kish. On the statistical analysis of noise in chemical sensors and its application for sensing. *Fluct. Noise Lett.* **01**, L147 (2001).
29. G. Scandurra, J. Smulko, L.B. Kish. Fluctuation-enhanced sensing (FES): A promising sensing technique. *Appl. Sci.* **10**, 5818 (2020).

Received 23.05.23.

Translated from Ukrainian by O.I. Voitenko

O.K. Видубіда

#### МАКСИМІЗАЦІЯ СЕЛЕКТИВНОСТІ ОЛЬФАКТОРНОГО РЕЦЕПТОРНОГО НЕЙРОНА В ПІДПОРОГОВОМУ РЕЖИМІ

Раніше було відомо, що представлення запахів ольфакторному рецепторному нейрону (ОРН) в підпороговій концентрації, тобто коли середнє значення кількості його зв'язаних рецепторних білків (РБ) недостатнє для генерації спайків, але така генерація все ж можлива завдяки флуктуаціям навколо середнього, селективність ОРН може бути вищою, ніж при вищих концентраціях і, зокрема, вищою, ніж у його РБ. У цій роботі для спрощеної моделі ОРН знайдено значення оптимальної концентрації для забезпечення найвищої селективності і виведено залежність найвищої селективності від повної кількості  $N$  РБ в ОРН і їх порогового значення  $N_0$ . Ефект покращення селективності в підпороговому режимі проявляється найкраще, коли  $N_0$  близьке до одиниці, або до  $N$ . Також він краще проявляється для більших  $N$ .

*Ключові слова:* ольфакторний рецепторний нейрон, селективність, підпороговий режим, флуктуації.
