# Supplementary material for: Selectivity gain in olfactory receptor neuron at optimal odor concentration
Source: arXiv:2504.10401 ancillary file (2025-04-14)
Supplement: Supplementary file 6 [file stoch_proc_simulation.pdf]

# Simulation of binding-releasing stochastic process

A.K.Vidybida\*

Bogolyubov Institute for Theoretical Physics, Kyiv, Ukraine

March 4, 2025

## Abstract

Here we describe how the process of binding-releasing of odor molecules with the set of ORs expressed in a single ORN is simulated in the program

## 1 Introduction

We characterize interaction of a single odor molecule (O1 or O2) with a single OR by means of two rate constants:

$k_+$  — is the odor binding rate (denoted in the program as `kp` for both O1 and O2);

$k_-$  — is the odor releasing rate (in the program: `km1`, or `km2` for O1, or O2),

which, together with odor concentration `c`, govern the following association-dissociation reaction:

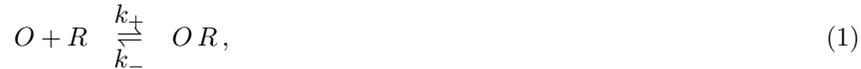

where  $R$  denotes the OR protein and  $O$  is either O1, or O2.

Suppose an ORN has  $N$  ORs at its surface. If an odor  $O$  is presented, then at any time  $t$ ,  $n(t)$  is the number of ORs which are bound with  $O$ , and  $N - n(t)$  are free. The physical meaning of  $k_+$ ,  $k_-$  is that  $c k_+ dt$  gives the probability that a free OR becomes bound during a small interval  $dt$ , and  $k_- dt$  gives the probability that a bound OR becomes free during the  $dt$ . Since the binding-releasing process is driven by the Brownian motion, the number  $n(t)$  changes randomly in time. In order to simulate with the time step  $dt$  ORN's activity in the odor presence, we need a realization (one of many possible) of the stochastic process:

$$\{n_0, n_1, \dots, n_k, \dots\}, \quad (2)$$

---

\*<http://vidybida.kiev.ua/>

where  $n_k \equiv n(k dt)$ . (In the program, the instant value of  $n$  at any time step is denoted as **n1**, or **n2** for odor O1, or O2, respectfully).

For small  $N$ , transition from  $n_k$  to  $n_{k+1}$  might be performed by calculating what happens with each OR during  $dt$ . To determine if a bound OR remains bound, produce a random number  $r$  from a uniform distribution in the interval  $[0; 1)$ . If  $r < pm$ , where

$$pm = k_- dt, \quad (\text{in the program: pm1, or pm2 for O1, or O2}) \quad (3)$$

then that OR becomes free, otherwise it remains bound. Similarly, for a free OR compare  $r$  with  $pp$ , where

$$pp = c k_+ dt, \quad (\text{in the program: pp, for both O1 and O2}). \quad (4)$$

If  $r < pp$  then that OR becomes bound, otherwise it remains free. Do this for all  $n_k$  bound and  $N - n_k$  free ORs and then calculate  $n_{k+1}$ .

Unfortunately, the number of ORs per ORN can be larger than  $10^6$ , [1]. Necessity to generate that much random numbers for each time step  $dt$  makes unfeasible a long simulation in a PC. But we need long simulations for several reasons. First, there are many (5000 - 10000) ORNs expressing the same OR protein, [2]. Repeating the same numerical experiment with different seeds will emulate a collective response in the set of ORNs expressing the same OR. Second, this simulation is of statistical nature and, to be reliable, it needs many repetitions with different seeds initializing the random number generators used.

## 2 Fast algorithm, theory

The sequence (2) is a realization of a Markov chain. Any realization of Markov chain can be produced with the help of its transition matrix:

$$p_{i,j} = p(j | i), \quad i = 0, \dots, N, \quad j = 0, \dots, N. \quad (5)$$

In our case,  $p(j | i)$  gives the probability to have  $j$  bound ORs at a time step, provided that at the previous time step there were  $i$  bound ORs. It is clear that

$$\sum_{j=0}^N p_{i,j} = 1 \quad \text{for any } i = 0, \dots, N.$$

In order to use  $p_{i,j}$  for generating a realization (2), calculate a new matrix  $P_{i,j}$  by the following way:

$$P_{i,j} = \sum_{j'=0}^j p_{i,j'}, \quad i = 0, \dots, N, \quad j = -1, 0, \dots, N. \quad (6)$$

A row  $\#i$  in the matrix  $P_{i,j}$  has the following form:

$$\{0, p_{i,0}, p_{i,0} + p_{i,1}, p_{i,0} + p_{i,1} + p_{i,2}, \dots, 1\}.$$

Now, to produce  $n_{k+1}$  following a given  $n_k$  in (2), produce a random number  $r$  from a uniform distribution in the interval  $[0; 1)$ , take the raw  $\#n_k$  in the  $P_{i,j}$ , find such  $j$  that

$$P_{n_k,j} \leq r < P_{n_k,j+1}, \quad (7)$$

and put

$$n_{k+1} = j + 1.$$

The matrix  $P_{i,j}$  is the same at any time step, and should be calculated in advance, before starting generation of realization (2). This can be done by the following way. First, considering binding-releasing events at different ORs as statistically independent, we calculate the transition matrix (5) as follows:

$$p_{i,j} = \sum_{f=\max(0,j-i)}^{\min(N-i,j)} BNkp(i, f+i-j, pm) BNkp(N-i, f, pp), \quad (8)$$

where  $f$  — is the number of ORs changing state from free to bound during  $dt$ , and  $(f+i-j)$  — is the number of ORs changing state from bound to free during  $dt$ , and

$$BNkp(N, k, p) = \binom{N}{k} p^k (1-p)^{N-k}, \quad k = 0, 1, \dots, N, \quad (9)$$

denotes a single term in a binomial distribution. Now, the required matrix  $P_{i,j}$  can be calculated as it is shown in (6).

### 3 Fast algorithm, implementation

#### 3.1 Starting from the mean

The mean in time number of bound ORs (either `nMEAN1`, or `nMEAN2` in the program) can be found as follows:

$$\text{nMEAN} = \text{p} * \text{N},$$

where `p` (in the program: `p1`, or `p2` for O1 and O2, respectfully) — is the probability to find any OR bound (in equilibrium occupancy, see sec. 3.4):

$$\text{p} = \text{N} * \text{kp} * \text{c} / (\text{kp} * \text{c} + \text{km}) \quad (10)$$

(in the program (files `init1.cpp` and `init2.cpp`), `km` is either `km1`, or `km2` for O1 and O2, respectfully). If we start simulation from `n0 = nMEAN`, then it is natural expecting that, for a long time (for the simulation time), the trajectory (2) will be confined in a some range `[nMIN; nMAX]` around the `nMEAN`, and not spanning all the possible for `n` values  $\{0, 1, 2, \dots, N\}$ . We choose (in the files `init1.cpp` and `init2.cpp`)

$$\begin{aligned} \text{nMIN} &= 0, \\ \text{nMAX} &= \text{nMEAN} + \text{nsig} * \text{sigma}, \end{aligned}$$

where the tunable parameter `nsig` is chosen in file `init.cpp`, and  $\sigma$  is the standard deviation for binomial distribution:

$$\sigma = \sqrt{Np(1-p)},$$

which is calculated as `sigma` in files `init1.cpp`, `init2.cpp` for O1 and O2, respectfully.

In the program, at each time step of the simulation it is checked that  $n \in [\text{nMIN}; \text{nMAX}]$ . Each case of violation of the last condition is reported in the calling terminal and is written to the report file `*.rep`. The values `nMEAN`, `nMIN` and `nMAX` are as well written to the report file for each of the two odors. For parameter values inspired by biological data it appeared that the number of possible  $n$  values within `[nMIN;nMAX]` is rather small compared with the total number  $N$  of ORs per ORN. This allows to reduce dimensions of matrices in (5) and (6), which, while drastically reducing the amount of necessary RAM, also makes the search task in (7) undemanding.

Actually, it is only necessary that initial value for  $n$  is chosen from the interval `[nMIN;nMAX]`, and to control that it remains there in the process of simulation. In the preliminary publication [3], we chose `nsig = 9` (in the file `init.cpp`). For this large value of `nsig`,  $0 \in [\text{nMIN}; \text{nMAX}]$ , and we chose  $n = 0$  at the beginning of each sniff in the simulation. Also, we chose `nMIN = 0` in the files `init1.cpp` and `init2.cpp` while calculating for [3].

## 3.2 Calculating matrix $P_{i,j}$

For calculating the matrix  $P_{i,j}$  we need the transition matrix, which can be calculated as it is shown in (8). Due to what is said in the Sec. 3.1, we need only a limited range of values for  $i, j$  in (8). This dictates the ranges for indices in the binomial terms used in the right hand side of (8). The first factor in (8) should be known for the indices

$$i = \text{nMIN}, \text{nMIN}+1, \dots, \text{nMAX}, \quad (f+i-j) = 0, 1, \dots, \text{nMAX}.$$

The second factor in (8) should be known for the indices

$$(N-i) = N-\text{nMAX}, \dots, N-\text{nMIN}, \quad f = 0, 1, \dots, \text{nMAX}.$$

### 3.2.1 Calculating necessary binomial terms

Firstly, we calculate those factors for the required ranges of indices. This is done in the files `make_BNkp_tabs1.cpp`, `make_BNkp_tabs2.cpp`.

Two tables are calculated for each odor. Each element in the 2D array `BNkp_pm1[ni][k]` defined in the file `make_BNkp_tabs1.cpp` and representing the first table gives the probability that exactly  $k$  ORs become free from  $\text{ni}+\text{nMIN}$

bound<sup>1</sup> during  $dt$ :

$$\text{BNkp\_pm1}[\text{ni}][\text{k}] = \binom{\text{ni}+\text{nMIN}}{\text{k}} \text{pm1}^{\text{k}} (1-\text{pm1})^{\text{ni}+\text{nMIN}-\text{k}},$$

$$\text{ni}=0, \dots, \text{nMAX}-\text{nMIN}, \text{k}=0, \dots, \text{nMAX}, \quad (11)$$

where  $\text{pm1}$  is defined in the file `init1.cpp` for the odor O1, and similarly for the second odor.

Each element in the 2D array `BNkp_pp1[i][k]` defined in the file `make_BNkp_tabs1.cpp` and representing the second table gives the probability that  $\text{k}$  ORs will become bound from  $\text{i}+\text{N}-\text{nMAX}$  free<sup>2</sup> during  $dt$ :

$$\text{BNkp\_pp1}[\text{i}][\text{k}] = \binom{\text{i}+\text{N}-\text{nMAX}}{\text{k}} \text{pp1}^{\text{k}} (1-\text{pp1})^{\text{i}+\text{N}-\text{nMAX}-\text{k}},$$

$$\text{i}=0, \dots, \text{nMAX}-\text{nMIN}, \text{k}=0, \dots, \text{nMAX}, \quad (12)$$

where  $\text{pp1}$  is defined as  $\text{pp}$  in the file `init.cpp` and used both in `init1.cpp` and `init2.cpp`. All four arrays (two for each odor) are saved in the directory `.probTabs` and used in further runs if possible.

### 3.2.2 Calculating $P_{i,j}$

The matrix  $P_{i,j}$  is presented in the files `make_fr_tabs1.cpp`, `make_fr_tabs2.cpp` by 2D arrays `fr1[dim1][dim1]`, where  $\text{dim1} = \text{nMAX1}-\text{nMIN1} + 1$  and similarly for the odor O2. We do not use in the program the case  $j = -1$ , which is shown in the Eq. (6) for explanation only.

As it was mentioned above, we suppose that, in the time course, the possible/expected number of bound ORs falls into the interval  $[\text{nMIN};\text{nMAX}]$  and check during simulation whether this restriction holds when the stochastic dynamics unfolds. In this case, in order to benefit from the restriction, we have to change the exact meaning of some elements in the `fr1[dim1][dim1]`. Namely, element `fr1[ni][0]` gives the probability that starting from  $\text{n}=\text{ni}+\text{nMIN}$  the next number  $\text{nn}$  of bound ORs belongs to the interval  $[0;\text{nMIN}]$ . This probability is extremely small. In order not to deal with vanishing probabilities we introduce a tunable parameter<sup>3</sup> `epsil` in the file `init.cpp`. If `fr1[ni][0] < epsil` then we put `fr1[ni][0] = 0`. The same is with the next elements `fr1[ni][1]`, `fr1[ni][2]`, ... until an element appears, which exceeds `epsil`. Also, if for some  $\text{nni}$  `fr1[ni][nni] > 1-epsil`, then we put `fr1[ni][nni] = 1`, and the same for all that follows  $\text{nni}$  up to  $\text{dim1}$ . This is justified since we check that the trajectory stays inside the interval  $[\text{nMIN};\text{nMAX}]$  during simulation.

When function `make_fr_tabs1()` finishes, array's element `fr1[ni][nni]`, if equal neither 0 nor 1, gives the probability that the number of bound ORs is

<sup>1</sup>Here, the number of bound ORs  $n = \text{ni} + \text{nMIN}$ .

<sup>2</sup>Here, the number of bound ORs  $n = \text{nMAX} - \text{i}$ .

<sup>3</sup>In this version we put `epsil = 0`, therefore the machine rounding does the job.

less or equal  $n_{ni} + n_{MIN}$  after passing a  $dt$  time step provided it was  $n_i + n_{MIN}$  before the  $dt$ . As a result, each row `fr1[ni] []` has the following form:

$$\{0, 0, \dots, 0, a, b, \dots, z, 1, \dots, 1, 1\}, \quad (13)$$

where  $0 < a < b < \dots < z < 1$ . The number of zeros and ones may vary from zero to several<sup>4</sup>. In the process of calculation we also create an array `n1r1[dim1][2]`, where `n1r[n][0]` and `n1r[n][1]` indicate position of the  $a$  and  $z$ , above (in the row  $\#n$ ). This is used further in the search task (7).

### 3.3 Finding the next $n$ ( $nn$ )

In the file `get_bound1.cpp` we generate a random number  $rn$  from a uniform distribution over  $[0; 1)$  and, having the current number  $n$  of bound ORs, decide which be the number of bound ORs,  $nn$ , at the next time step. For this purpose it is necessary to find the right place for  $rn$  within the row `fr1[n-nMIN] []` exemplified in (13). This is done in the file `get_place1.cpp` in the following manner. If  $a \leq rn < z$  then we do the standard search as required in (7). In highly improbable cases when either  $rn < a$  or  $rn \geq z$  we put either  $nn=n_{MIN}$  or  $nn=n_{MAX}$ , respectfully, and report the total number of such unlucky cases in the report file and in the calling terminal. For the parameters chosen here (mainly,  $n_{sig} = 9$ ) we have not observed the unlucky cases at all.

Proceeding as described above, we generate the entire stochastic trajectory (2) for both O1 and O2 during the time interval `sniffDur`, which is specified in the file `DATA.RUN`.

### 3.4 Checking the binomial distribution

In the file `get_bound1.cpp`, a vector type container `distrib1` accumulates data about occurrences of each number  $n$  of bound receptors. When the trajectory is through, `distrib1[ni]` gives the number of time steps at which the number of bound ORs was exactly  $n = n_i + n_{MIN}$ , and similarly for the second odor. Having the `distrib1` complete, we check whether the set of numbers `distrib1[ni]` complies with the binomial distribution with parameters  $N, p$ , where  $p$  is given in (10). The check is made by calling `check_binomial1()` in the file `run_trajec1.cpp`, and similarly for O2. In this version, the call is commented out. Uncomment it for doing the check.

It should be taken into account that even for a very long simulation, cases of the  $n$  being close to  $n_{MIN}$  or  $n_{MAX}$  are extremely rare. Their probability cannot be reliably determined in a numerical experiment. Therefore, we exclude those cases from the check. For this purpose, a parameter `tolera = 0.1` is introduced in the `init.cpp`. Cases having a total probability, that is calculated with a true binomial distribution, less than `tolera` are excluded from testing.

<sup>4</sup>Uncomment the ‘`//#define type_fr`’ line in the file `type.in.terminal.h` to see an example of raws in the `fr[] []`.

## References

- 1 K-E Kaissling. Olfactory perireceptor and receptor events in moths: A kinetic model. *Chemical Senses*, 26:125–150, 2001.
- 2 K. J. Ressler, S. L. Sullivan, and L. B. Buck. Information coding in the olfactory system: evidence for a stereotyped and highly organized epitope map in the olfactory bulb. *Cell*, 79:1245–1255, 1994.
- 3 A. Vidybida. Selectivity gain in olfactory receptor neuron at optimal odor concentration. In *2024 IEEE International Symposium on Olfaction and Electronic Nose (ISOEN)*, pages 1–3, 2024.
